# Supplementary material for: What Are Tools Anyway? A Survey from the Language Model Perspective
Source: arXiv:2403.15452 source file (2024-03-18)
Supplement: Supplementary file 1 [file embodied.tex]

\section{Tools with embodied agents}
\label{sec:embodied}

\zwcomment{merge related works to earlier sections and remove this section?}

In previous sections, we discuss LM-used tools in NLP task environments. In the last part of this survey, we broaden our discussion about tools to the agent-environment interaction setup. 
Specifically, we regard \emph{agents} as the policies that interact with environments based on the perceived environmental state;\footnote{We are specifically interested in LM-based agents, which use LM as a component.} and \emph{environments} are the collections of objects and their relationships.\footnote{In NLP tasks, an environment contains example contexts and the collection of tool environments.}
While most objects can be purposed as tools, e.g., brushes can be used to paint, brooms can reach high objects, % magnifiers can help read books,
% books can be used to hit nails into blocks, terminal can be used to execute a drawing program, 
the following definition captures the essence of tools:

\begin{definition}[Tools]
\label{def:tools_broad}
Tools are the objects in the environments that are not directly part of the goals of the agents, but are used by the agents in order to achieve the goals.
\end{definition}

For example, when drawing a picture, $\{$brush, paint, canvas$\}$ are all used, but only the \texttt{brush} is regarded as tools, since they are not part of the final product --- a picture.
% \zwcomment{we could align what figure 4 draws to the examples we made below. it also helps that you could discuss the example by referring to the illustration}
% For example, when making a hamburger, stove, toaster, pans, breads, patties, tomatoes, and cabbages are all used, but only stove, toasters, and pans are regarded as tools, since they are not part of final product, a hamburger. 
It should be noted that an object can be a tool for one task but not a tool for another, e.g. a \texttt{calculator} is a tool when finding the root of an equation, but it is not a tool when a virtual agent is launching the calculator app.\footnote{The definition of tools used by humans and non-human animals has been evolving in the past decades. Def. \ref{def:tools_broad} is similar to \citet{beauchamp2011oxford}, which defines tools as inanimate objects ``causing a change in the environment, thereby facilitating one's achievement of a target goal''.}

\begin{wrapfigure}[18]{r}{0.43\textwidth}
\vspace{-4mm}
\footnotesize
    \includegraphics[width=0.43\textwidth]{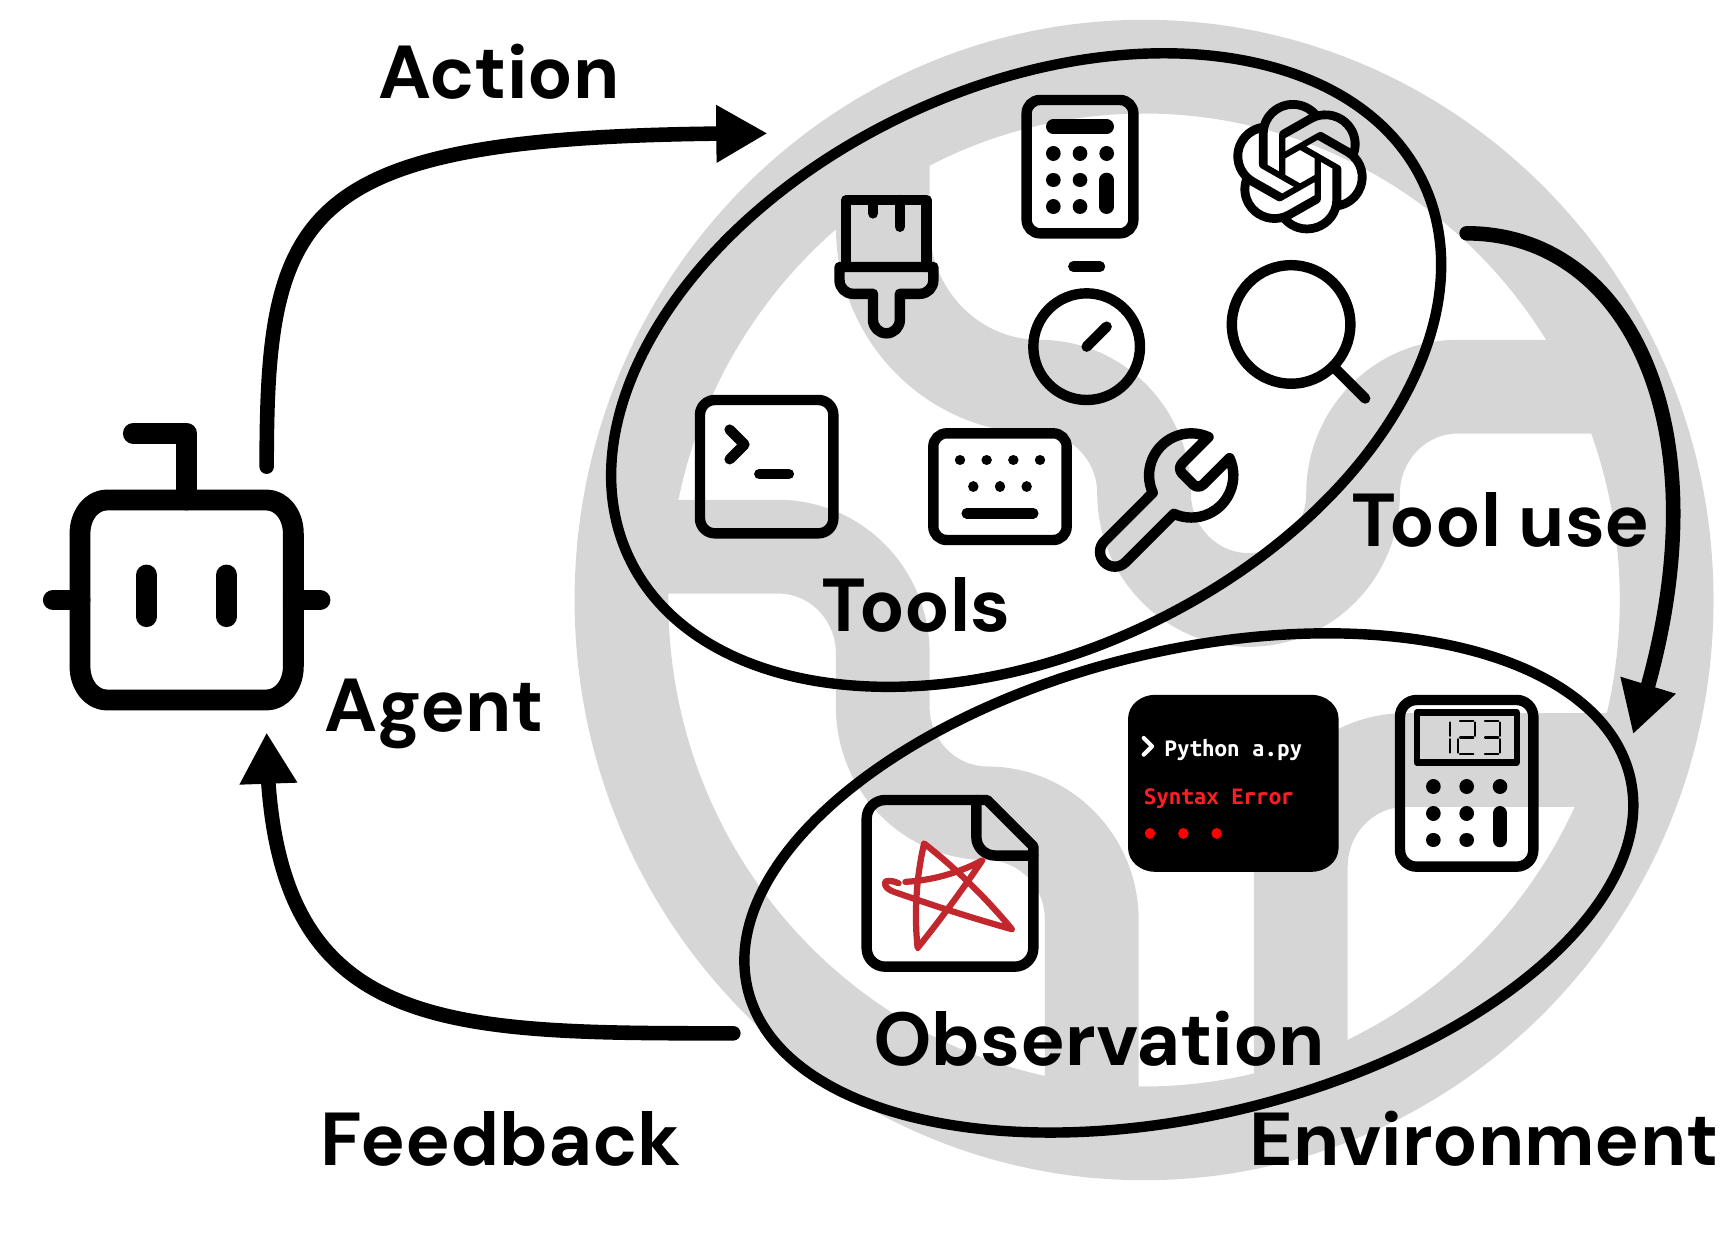}
\vspace{-6mm}
\caption{The action-observation feedback loop: an agent interacts with an environment by acting (with tools) on other objects in the environment, and getting feedback reward from it.}
\label{fig:agent-env}
\end{wrapfigure}

The approaches for using tools under Def. \ref{def:tools-lm} can also be applied to tools under Def. \ref{def:tools_broad}, by implementing external functions composed of low-level manipulation policies. 
These composed functions are often \textit{rule-based methods} or \textit{magic functions} provided by the simulation environments (similar to works providing expert-designed APIs to LMs in \S\ref{sub:app-spec}). For example, \citet{shridhar2020alfred} employ human-crafted APIs in the AI2THOR simulator \citep{kolve2017ai2} to use microwaves and fridges to cool and heat objects.  
\citet{wang2023voyager} use JavaScript APIs in Mineflayer\footnote{\url{https://github.com/PrismarineJS/mineflayer}} to manipulate Minecraft tools such as mining with axes. \citet{liu2024agentbench} hand-craft the \texttt{search} tool as Python functions to query data over the web, and \citet{boiko2023autonomous} similarly for conducting chemical research.

However, in the real world, not all high-level manipulation policies are readily available. For example, in \citet{ahn2022saycan}, % although picking up sponges can be learned as a policy, 
wiping tables with a sponge is too complex to be implemented as an action, hence is actually executed by humans.
% although picking up sponge is a learned subpolicy, wiping tables with a sponge is executed by humans. 
Nonetheless, instead of adopting readily available policies, these compositions can also be learned via behavior cloning and reinforcement learning.
For instance, \citet{baker2019emergent} show that tool use can be learned without expert demonstrations or rewarding signals, and \citet{yu2023language} feed NL inputs to robots to learn skills such as picking up apples.
% More recently, \citet{ahn2022saycan} also learn policies to pick up objects such as sponges.

Training and evaluating LMs and LM-based agents on their tooling abilities in the real world remain an open challenge.
% Training and evaluating LMs' and LM-based agents' ability to use tools in the real world remains an open question. 
Here we highlight two future directions: (1) \textit{building more complex environments}: with sufficient objects for versatile tool use and tool make, (2) \textit{harness LM procedural knowledge}: LMs equip strong procedural knowledge via extensive training, which can be utilized to improve planning and navigation in complex, realistic environments.
